# Supplementary material for: LLM4GEN: Leveraging Semantic Representation of LLMs for Text-to-Image Generation
Source: arXiv:2407.00737 source file (2024-08-27)
Supplement: Supplementary file 1 [file appendix.tex]

\title{Supplementary Materials: LLM4GEN: Leveraging Semantic Representation of LLMs for Text-to-Image Generation}

\section{Additional Analysis}
We provide the additional analysis and experimental results on our proposed LLM4GEN in the Supplementary Materials.

\textbf{Formualtion Derivation}
We provide a formula derivation of Eq.~(8): 
\begin{equation}
\begin{aligned}
x &= \operatorname{CA}(x, c_t') \\
&= \operatorname{softmax}\left(Q' \cdot {K'}^T\right) \cdot V' \\
&= \operatorname{softmax}\left(W_Q'(x) \cdot {W_K'(c_t')}^T\right) \cdot W_V'(c_t') \\
&= \operatorname{softmax}\left(W_Q'(x) \cdot {W_K'([\lambda \cdot c_l', c_t])}^T \right) \cdot W_V'([\lambda \cdot c_l', c_t]) \\
&= \lambda \cdot \operatorname{softmax}\left(W_Q'(x) \cdot {W_K'(c_l')}^T\right) \cdot W_V'(c_l') \\
&\quad + \operatorname{softmax}\left(W_Q'(x) \cdot {W_K'(c_t)}^T\right) \cdot W_V'(c_t) \\
&= \lambda \cdot \operatorname{CA}(x, c_l) + \operatorname{CA}(x, c_t)
\end{aligned}
\end{equation}

where $x$ denotes the latent noise, \text{CA} is the cross-attention module within the UNet module, which receives $z$ as the query and $c_t'$ as the key and value. And the $W_Q', W_K', W_V'$ is the projector in the UNet. In this manner, the concatenation operation in Eq.~(7) is equal to fuse the LLM-guided semantic feature to the latent noise for better text-to-image alignment.

\textbf{Algorithm.} The proposed LLM4GEN is further illustrated in \cref{algorithm: llm4gen}.

\begin{algorithm}[!h]
\caption{LLM4GEN Pipeline}
\begin{algorithmic}[1]
\STATE \textbf{Input: } Pretrained UNet $\epsilon$, pre-trained text encoder $T_\phi$, pre-trained LLM $T_{L}$, Cross-Adapter Module $M$, LLaVA-7B $A$, training image-text pairs $\mathbb{S} = \{\mathbb{I}, \mathbb{P}\}$ .
\STATE \textbf{Offline Process: } Apply $A$ to enrich the captions of $\mathrm{S}$, get $\hat{\mathbb{P}}$ = $A$($\mathrm{I}$) to replace the original $\mathbb{P}$. 
\STATE $\rightarrow$ \textbf{Begin Training.}
\STATE Freeze $T_\phi$ and $T_{L}$, training $M$ and $\epsilon$.
\WHILE{${L_{simple}}$ not converged}
    \STATE Sample $p$ from $\mathbb{P}$; $t = T$
    \STATE ${c_{t}'} = M(T_{\phi}(p), T_{L}(p))$ using Eq.~(7).
    \STATE Calculate ${L_{simple}}$ using Eq.~(9).
    \STATE Backward ${L_{simple}}$ and update $\epsilon$, $M$.
\ENDWHILE
\STATE $\rightarrow$ \textbf{End Training.}
\end{algorithmic}
\label{algorithm: llm4gen}
\end{algorithm}

\begin{figure}[!ht]
    \centering
    \includegraphics[width=\linewidth]{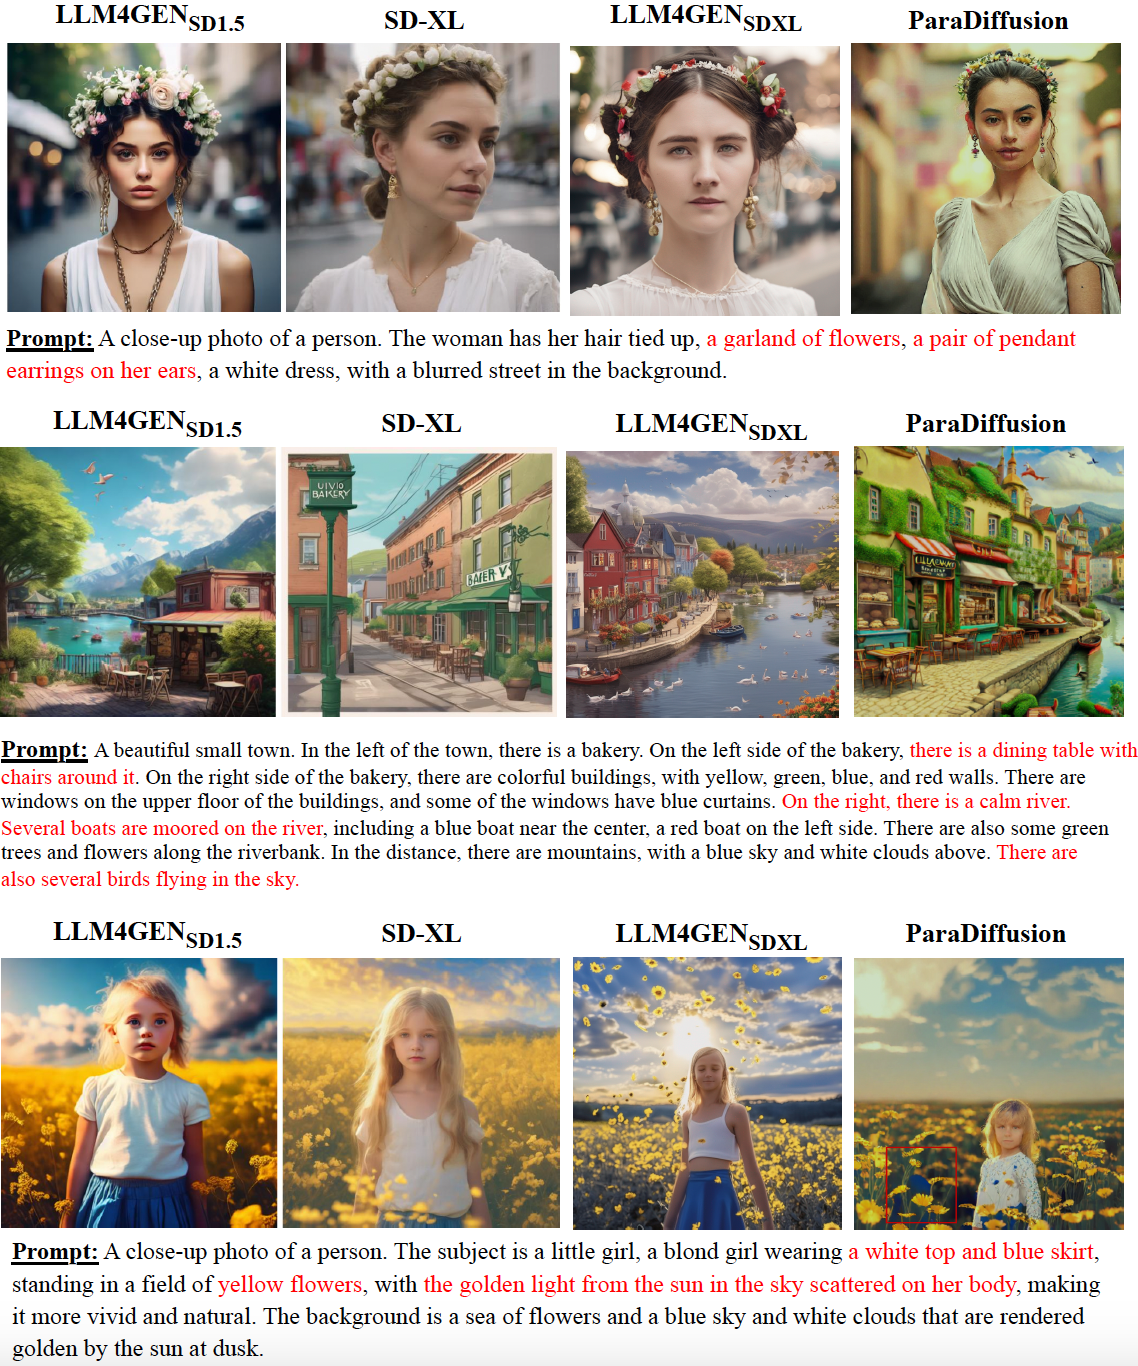}
    \caption{Comparison with ParaDiffusion \cite{wu2023paragraph}. The generation images of ParaDiffusion are from the original paper.}
    \label{fig:paradiffusion}
\end{figure}

\begin{figure}[!ht]
    \centering
    \includegraphics[width=\linewidth]{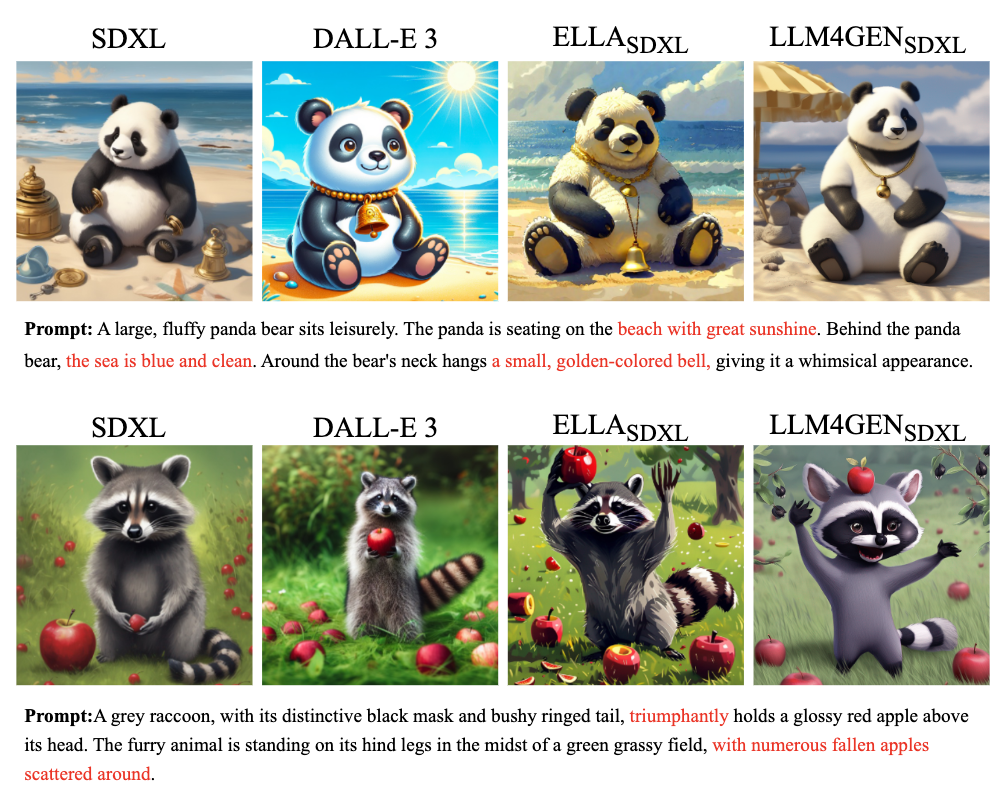}
    \caption{Comparison with ELLA \cite{ella}. The generation images of ParaDiffusion are from the original paper.}
    \label{fig:ella}
\end{figure}

\section{Additional Experimental Results}

\begin{figure}[!ht]
    \centering
    \includegraphics[width=0.9\linewidth]{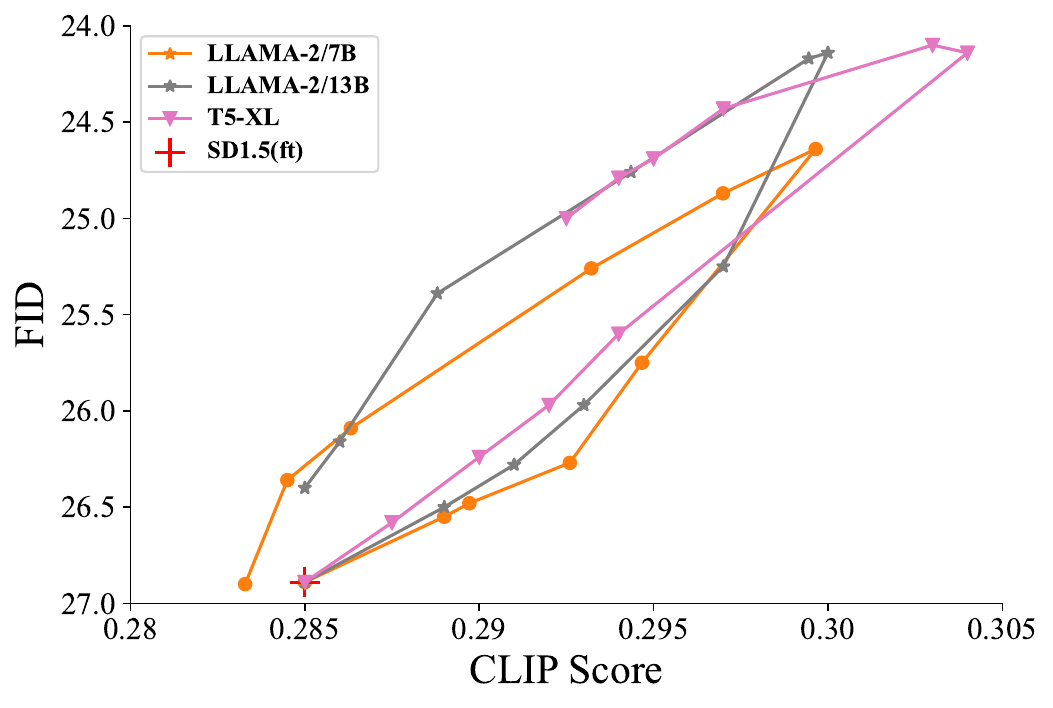}
    \caption{Performance metrics of LLM4GEN based on different LLMs across $\lambda$ values from 0 to 2.}
    \label{fig:lambda}
\end{figure}

% Optional
\textbf{Impact of hyperparameter $\lambda$.} As depicted in \cref{eq:e1}, the hyperparameter $\lambda$ is used to regulate the weight of the LLM's embedding injected into the original text embedding. We evaluate the impact of $\lambda$ in \cref{fig:lambda} with FID and CLIP Score for LLM4GEN$_{SD1.5}$ on MSCOCO dataset across different LLMs. The $\lambda$ varies from 0 to 2 in 0.2 increments. As the $\lambda$ increases, we observe an initial enhancement in the model's performance, followed by a slight decline. This pattern indicates that integrating LLMs representation into that of the original text encoder can consistently improve the image-text alignment beyond the capabilities of the original SD1.5, highlighting the beneficial impact of LLMs on semantic enrichment. However, setting higher values of $\lambda$ does not lead to optimal performance, which we suspect stems from a misalignment between LLMs representation and the diffusion model. The best performance is achieved when $\lambda$ is set to 1.0.

\textbf{Comparison with ParaDiffusion based on dense prompts.} To further compare the proposed LLM4GEN with ParamDiffusion, we take three prompts provided in \cite{wu2023paragraph}, and generate images using our LLM4GEN$_{SD1.5}$ and LLM4GEN$_{SDXL}$.  We select the generation images of ParaDiffusion from the original literature \cite{wu2023paragraph}. The results demonstrate that our proposed LLM4GEN can generate semantic-alignment images based on long textual descriptions and alleviate bad cases in ParaDiffusion, such as confusion between character generation and background in \cref{fig:paradiffusion}~(c). LLM4GEN$_{SD1.5}$ even can generate high-quality and dense prompts alignment images than SDXL\cite{podell2023sdxl}, such as \cref{fig:paradiffusion}~(b). It demonstrates our proposed methods can efficiently integrate strong semantic representations of LLMs into text-to-image diffusion models to enhance image-text alignment.

\textbf{Comparison with ELLA \cite{ella}.} ELLA \cite{ella} also utilizes LLMs for text-to-image generation, with the aim of aligning LLMs with diffusion models from scratch, incurring significant training costs. In contrast to ELLA, our proposed LLM4GEN enhances the original text encoder directly with robust LLM semantic embeddings. This approach benefits from the powerful capabilities of LLM without high-cost training and computing sources. Compared to ELLA$_{SDXL}$, our model requires only 10\% of the training data, but still produces high-quality images using the prompts provided in \cite{ella}. The visualization comparison is presented in \cref{fig:ella}. 

\begin{figure}[!ht]
    \centering
    \includegraphics[width=\linewidth]{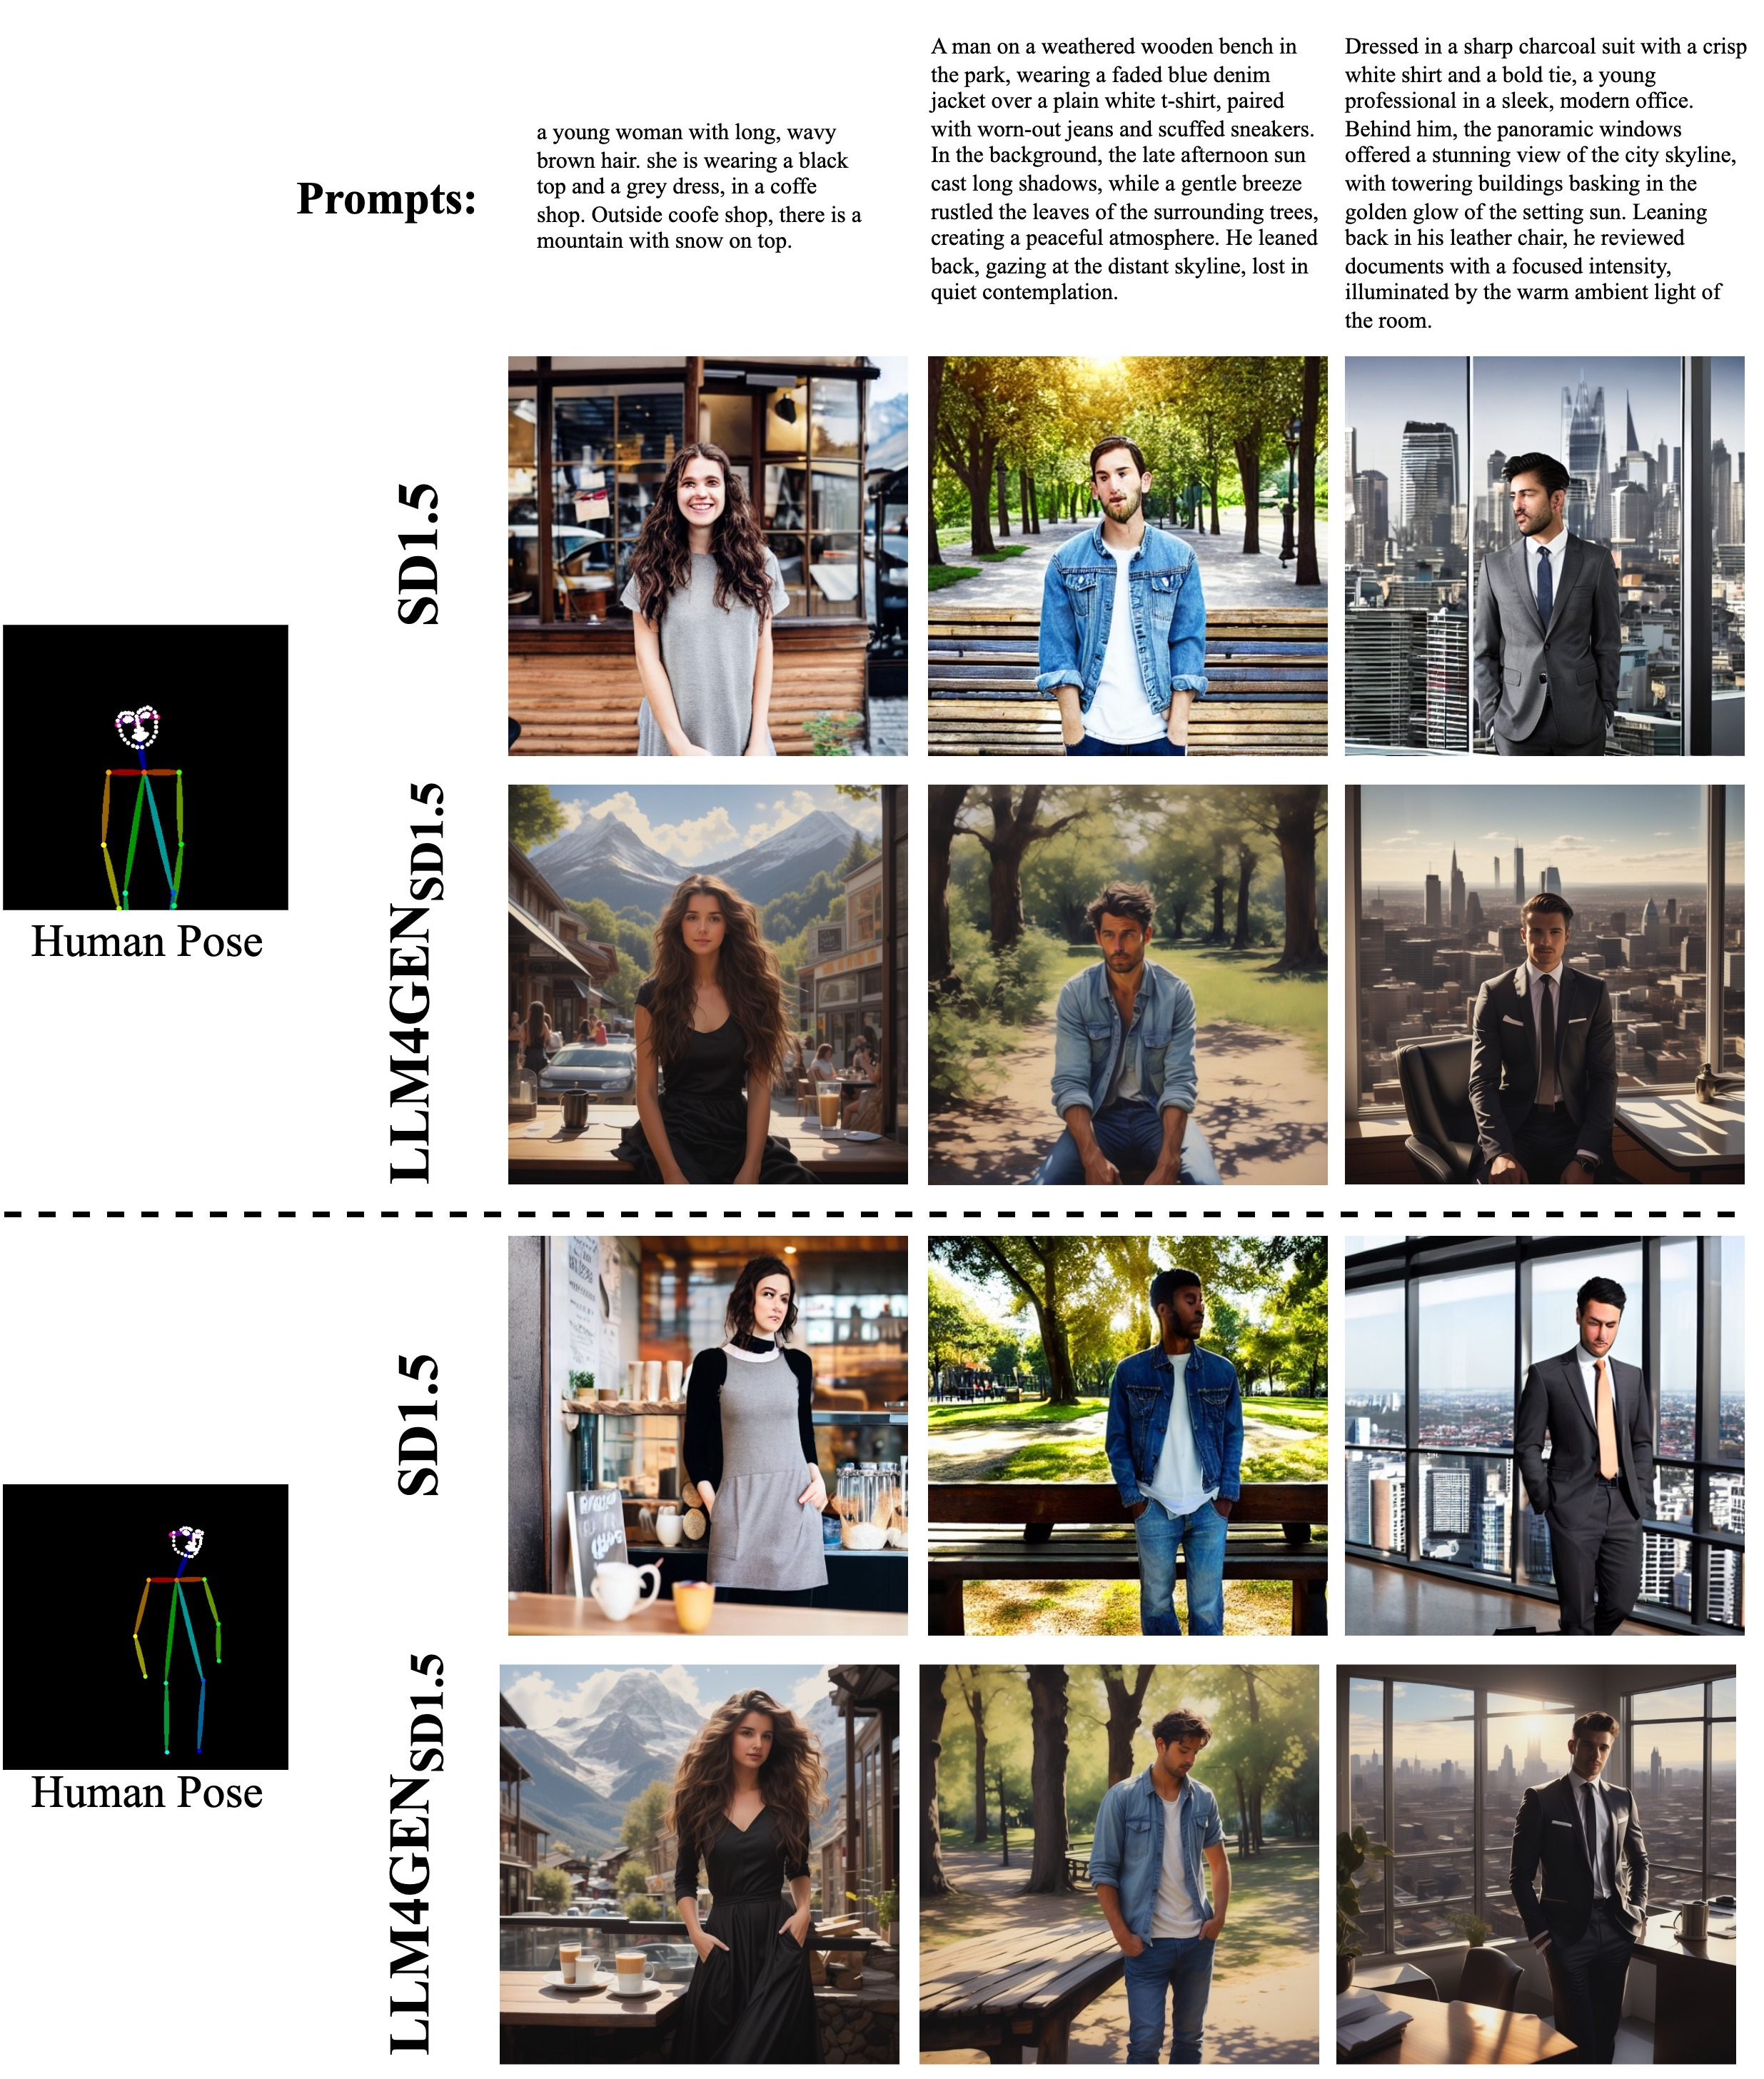}
    \caption{LLMGEN$_{SD1.5}$ can be integrated with ControlNet \cite{controlNet} to generate images with guided poses.}
    \label{fig:controlnet}
\end{figure}

\textbf{Compatible with ControlNet \cite{controlNet}.} We apply LLM4GEN with ControlNet  \cite{controlNet}, as shown in \cref{fig:controlnet}. We can see that LLM4GEN$_{SD1.5}$ can be integrated with exsiting guided tools like ControlNet.  LLM4GEN$_{SD1.5}$ can be compatible with these standard methods while generates more consistent and text-align images.
